# Supplementary material for: Processing Analytical Workloads Incrementally
Source: arXiv:1509.05066 source file (2015-09-16)
Supplement: Supplementary file 1 [file appendixA.tex]

Let $D$ be the underlying data set of $n$ points. A point $p \in D $ is represented as $p= (id,y,x)$, where $id$ is the identifier, $y$ the dependent (class) variable and $x$ the feature vector as defined before. Let $D_1$ and $D_2$ be two Naive Bayes model with corresponding model descriptors represented by $d(D1) = [a_1,b_1] $ and $d(D2)  =  [a_2,b_2]$.   Our  aim  is  to  compute  the Naive Bayes model for $D_u = D_1 \cup D_2$. For each materialized models we maintain the following information 
$N_c$, $S_{jc}$ and $SS_{jc}$ as discussed in section \ref{subsec:NB}. Combining the two Naive Bayes model $D_1$ and $D_2$ involves considering two cases : \textit{Case 1:} The two datasets do not overlap i.e. $D_1 \cap D_2 = \phi$; which can be easily identified by comparing model descriptors for $D_1$ and $D_2$. The model $D_u$ can be materialized using the following equations 

\begin{displaymath}N_c^u = N_c^1 + N_c^2\end{displaymath}
\begin{displaymath}S_{jc}^u = S_{jc}^1 + S_{jc}^2\end{displaymath}
\begin{displaymath}SS_{jc}^u = SS_{jc}^1 + SS_{jc}^2\end{displaymath}

\textit{Case 2:} The two data sets have points in common i.e. $D_1 \cap D_2 \neq \phi$; the points common to both data sets can be  determined  from  the  corresponding  model  descriptors. We can compute the materialized model $D_u$ along same lines as case 2 in section \ref{subsec:lrm} 

\begin{displaymath}N_c^u = N_c^1 + N_c^2 - \sum_i^{D_1 \cap D_2}[y^{(i)}=c] \end{displaymath}
\begin{displaymath}N_c^u = N_c^1 + \sum_i^{D_2 - D_1}[y^{(i)}=c] \end{displaymath}
\begin{displaymath}N_c^u = N_c^2 + \sum_i^{D_1 - D_2}[y^{(i)}=c] \end{displaymath}
%\begin{displaymath}S_{jc}^u = S_{jc}^1 + S_{jc}^2 - \sum_i^{D_1 \cap D_2}x_j^{(i)}[y^{(i)}=c]\end{displaymath}
%\begin{displaymath}SS_{jc}^u = SS_{jc}^1 + SS_{jc}^2 -  \sum_i^{D_1 \cap D_2}(x_j^{(i)}[y^{(i)}=c])^2 \end{displaymath}

$S_{jc}^u$ and $SS_{jc}^u$ can also be computed in a similar fashion.
