# Supplementary material for: Processing Analytical Workloads Incrementally
Source: arXiv:1509.05066 source file (2015-09-16)
Supplement: Supplementary file 2 [file appendixB.tex]

In this section we wish to establish a bound for the model parameter calculated by Algorithm \ref{algo:psgd} . The bound obtained below holds true for any model with convex and differentiable loss
function. Let $X$ denote the feature vector space and $Y$ the output space, and  $\Phi : X \times Y  \rightarrow H$  a (feature) mapping to a Hilbert space $H$, which in many practical settings coincides with 
$\mathbb{R}^N , N = dim(H) < \infty $. The norm induced by the inner product associated with the hilbert space $H$ is represented by $\| \ \|$.
Let $S = ((x_1, y_1), . . . ,(x_m, y_m))$ be a training sample of $m$ tuples in $X \times Y$. A conditional maximum entropy model has
a conditional probability of the form $p_w[y|x]= \frac{1}{Z(x)}exp(w·\Phi(x, y))$ 
with $Z(x)= \sum_{y∈Y} exp(w·\Phi(x, y))$, where the weight or parameter vector $w\in H$ is the solution of the following optimization problem:
\begin{displaymath}
w = \underset{w \in H}{\operatorname{argmin}} \ F_S(w) = \underset{w \in H}{\operatorname{argmin}} \ \lambda {\| w \|}^2 - \frac{1}{m}\sum_{i=1}^{m}log \ p_w[y_i|x_i] 
\end{displaymath}

where $\lambda$ is a regularization parameter. Let $z = (x,y) \in X \times Y$ denote a training sample and $L_z(w) = -log p_w[y|x]$ is the negative log-likelihood.
Let $S$ and $S^{'}$ be two training sample of size $m$ which differ at one point, $S = (z_1, . . . , z_{m−1}, z_m)$ and $S^{'} = (z_1, . . . , z_{m−1}, z_m^{'})$. Let $w$ and $w^{'}$ be the parameter vector obtained
after training on sample $S$ and $S^{'}$ respectively. Let $\Delta w $ be denoted as $w^{'} - w$. We assume that the feature vectors are bounded, $\exists R > 0 $ such that $ \forall (x,y) \in X \times Y $, 
$\| \Phi(x,y) \| \leq R$.

\begin{theorem}
Let $S^{'}$ and $S$ be two arbitrary samples of size m differing only by one point. Then, the following stability bound holds for the weight vector returned by a conditional maxent model:
\begin{displaymath}
\| \Delta \| \leq \frac{2R}{\lambda m}
\end{displaymath}
\end{theorem}

the above theorem can be proved using constructs of Bregman divergence and applying Cauchy-Schwarz inequality. 
Let $D$ denote the true distribution according to which 
training and test points are drawn. Let $F^*$ be the associated loss function and $ w^* = \underset{w \in H}{\operatorname{argmin}} \ F^*(w)$.

\begin{theorem}
Let $w \in H$ be the weight vector returned by conditional maximum entropy when trained on a sample $S$ of size $m$. Then, for any $\delta > 0$, with probability at least $1 - \delta$, the following inequality holds:
\begin{displaymath}
\| w - w^* \| \leq \frac{2R}{\lambda \sqrt{m/2}}(1+\sqrt{log1/\delta})
\end{displaymath}
\end{theorem}

The above result is independent of the dimension of the feature space and depends only on R the radius of the sphere containing the feature vectors.
Consider now a sample $S = (S_1, . . . , S_{pm})$ of $pm$ points formed by $p$ subsamples of size $m$ points drawn i.i.d. and let $w_{\mu}$ denote the parameter derived using Algorithm \ref{algo:psgd}. The following theorem gives a bound for $w_{\mu}$.

\begin{theorem}
For any $\mu \in \Delta_{p}$, let $w_{mu} \in H$ denote the mixture weight vector obtained from a sample of size $pm$ by combining the $p$ weight vectors $w_k$, $k∈[1, p]$, each returned by conditional maximum
entropy when trained on the sample $S_k$ of size $m$. Then, for any $\delta >0$, with probability at least
$1 - \delta$,
the following inequality holds:
\begin{displaymath} \| \vec{w_{\mu}} - \vec{w^*} \| \leq E[\| \vec{w_{\mu}} - \vec{w^*} \|]  + \frac{R \| \mu \| }{\lambda\sqrt{m/2}}\sqrt{log1/\delta} \end{displaymath}
\end{theorem}

For a uniform mixture the norm is given by $\| \mu \| = \frac{1}{\sqrt{p}}$. We can bound the term $E[\| \vec{w_{\mu}} - \vec{w^*} \|]$ by applying the triangle inequality. 

\begin{displaymath}
E[\| w_{\mu} - w^* \|] = E[\| \frac{1}{p} \sum_{k=1}^{p} ( w_k - w^{*} ) \|] \leq E[\| w_{1} - w^{*} \|]
\end{displaymath}

Thus using Theorems 2 and 3 we can compare the parameter $w_{pm}$ obtained by training on a sample of size $pm$ versus the mixture of weight parameter $w_{\mu}$ for the same sample.
